# Supplementary material for: New insights on carbon black suspension rheology -- anisotropic thixotropy and anti-thixotropy
Source: arXiv:2202.05772 ancillary file (2022-02-09)
Supplement: Supplementary file 1 [file CB_thixo_OSP_SI_2022-02-08.pdf]

# New insights on carbon black suspension rheology - anisotropic thixotropy and anti-thixotropy
# Supporting Information

Y. Wang[1,2,3] and R. H. Ewoldt[1,2,3,4,a)]

[1)] *Department of Mechanical Science and Engineering, University of Illinois at Urbana-Champaign, Urbana, Illinois 61801, USA*

[2)] *Beckman Institute for Advanced Science and Technology, University of Illinois at Urbana-Champaign, Urbana, Illinois 61801, USA*

[3)] *Joint Center for Energy Storage Research, Argonne National Laboratory, Lemont, Illinois 60439, USA*

[4)] *Materials Research Laboratory, University of Illinois at Urbana-Champaign, Urbana, Illinois 61801, USA*

(Dated: 8 February 2022)

[a)] Author to whom correspondence should be addressed; electronic email: ewoldt@illinois.edu

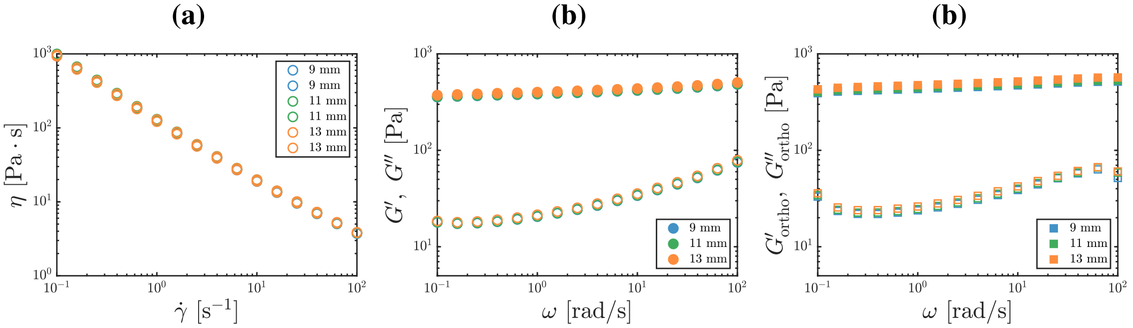


FIG. 1. Verify the consistency of measurements using OSP geometry at different operating heights using Carbopol 940: (a) the steady state shear viscosity, $\eta$, as a function of applied shear rate, $\dot{\gamma}$, (b) the rotational moduli, $G'$ and $G''$, as a function of frequency, $\omega$, and (c) the orthogonal moduli, $G'_{\perp}$ and $G''_{\perp}$, as a function of frequency.

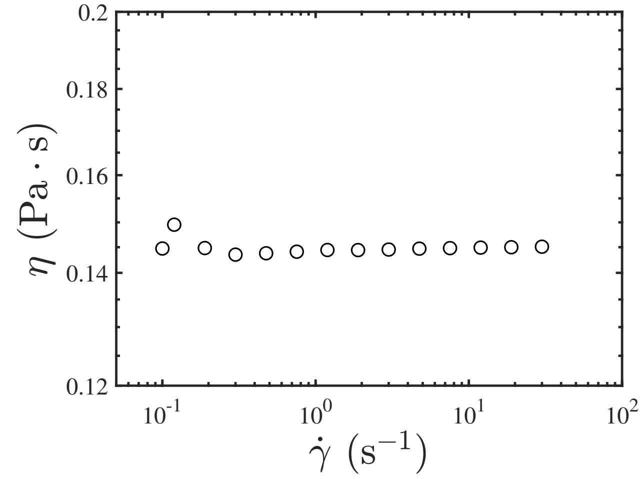


FIG. 2. The steady state viscosity as a function of applied shear rate of heavy mineral oil, which is the solvent for CB suspensions used in this study.

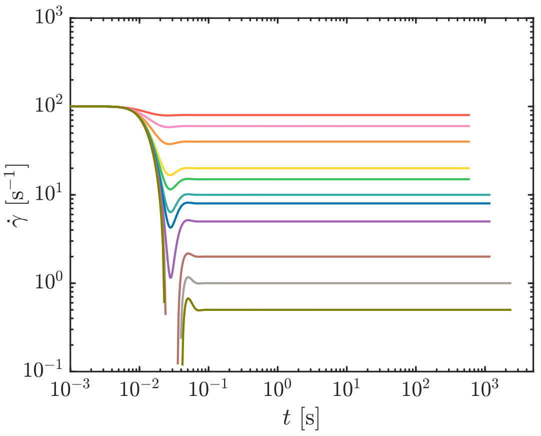


FIG. 3. The transient shear rate input during the step-down shear tests with initial shear rate of 100 s$^{-1}$ and final shear rate ranging from 80 to 0.5 s$^{-1}$ for a 6 wt% CB suspension: the motor reaches steady state shear rate in around 50 ms.

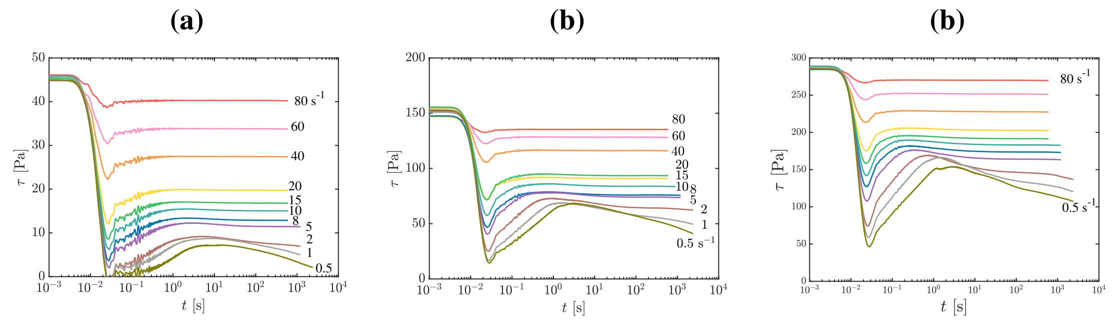


FIG. 4. The transient stress measured during the step-down shear tests with initial shear rate of 100 s$^{-1}$ and final shear rate ranging from 80 to 0.5 s$^{-1}$ for CB suspensions of (a) 4 wt%; (b) 8 wt%; and (c) 10 wt%. A peculiar, combined short-time recovery and long-time decay dynamics is observed at the lower shear rate conditions for all concentrations.

The period of oscillation in Fig. 3 is $T_o = 0.02$ s, therefore, the frequency of oscillation is: $f_{\mathrm{o}} = 50$ Hz.

The angle of the cone-and-plate geometry, $\beta$, is 0.1 rad, giving the geometry-dependent conversion factor of $F_\gamma = \frac{1}{\beta} = 10$. For shear rate ranging from 1 to 100 s$^{-1}$, the rotational velocity is ranging from $\omega = 0.1$ to 10 rad/s, therefore, the motor rotating frequency, $f_{\mathrm{r}}$ is 0.016 to 1.6 Hz.

For viscoelastic wave propagation, the wavelength of the linear viscoelastic shear wave between a moving boundary and a fixed reflecting boundary is[1]

$$l = \frac{1}{\cos(\delta/2)} \left( \frac{|G^*|}{\rho} \right)^{1/2} \frac{1}{f_w}, \tag{1}$$

where $\delta$ is the viscoelastic phase angle, $G^*$ is the complex modulus, $\rho$ is the fluid density, and $f_w$ is the wave frequency. If the viscoelastic wave is why we observed oscillations in data during shear, the wavelength is $l = d = R\tan\beta \sim 0.218$ mm, where $R$ is the radius of the geometry, $\cos(\delta/2) \sim 1$, $|G^*| \sim 500$ Pa, and $\rho \sim 1800$ kg/m$^3$, and this gives the wave frequency $f_{\mathrm{w} \sim 2400\ \mathrm{Hz}}$.

The mismatch between the oscillation frequency, $f_o = 50$ Hz, the rotating frequency, $f_r$ is 0.016 to 1.6 Hz, and the viscoelastic wave frequency, $f_w \sim 2400$ Hz, suggests that the stress oscillation is not a result of uneven sample loading nor viscoelastic wave.

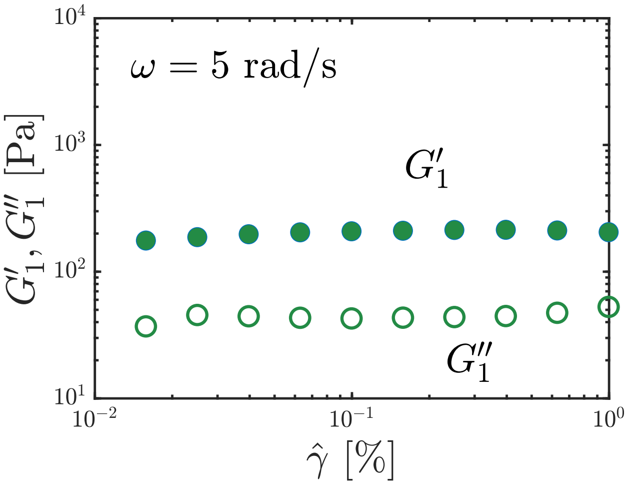


FIG. 5. The large amplitude oscillatory shear (LAOS) results of 6 wt% CB suspension at frequency of 5 rad/s: the suspension remains linear up to amplitude of 1%.

## REFERENCES


[1]R. H. Ewoldt, M. T. Johnston, and L. M. Caretta. *Experimental challenges of shear rheology: how to avoid bad data, in: Complex fluids in biological systems*. Springer Biological Engineering Series, 2015.

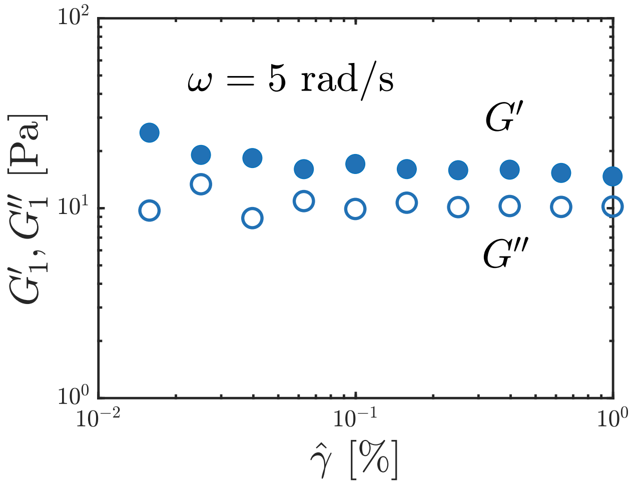


FIG. 6. The large amplitude oscillatory shear (LAOS) results of 4 wt% CB suspension at frequency of 5 rad/s: the suspension remains linear up to amplitude of 1%.

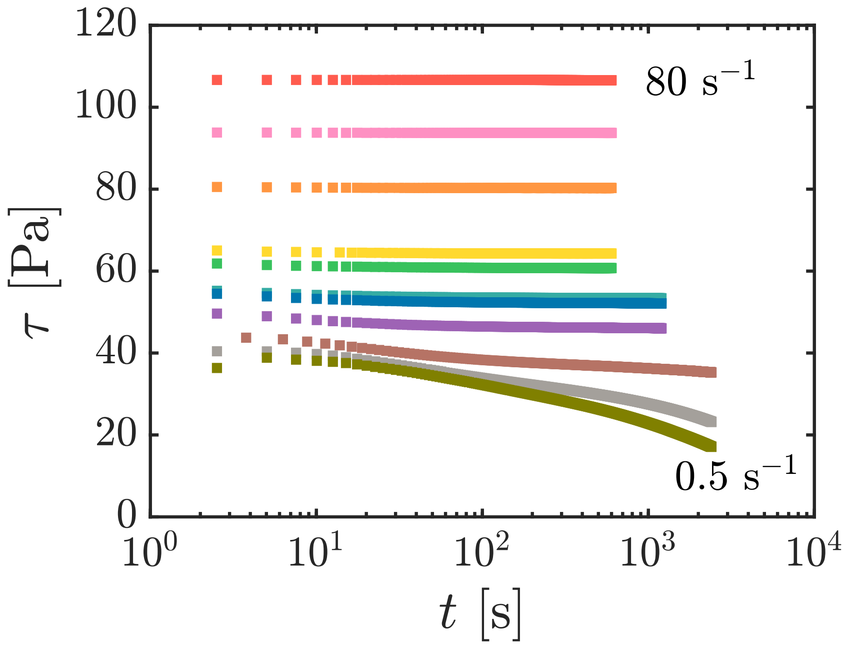


FIG. 7. The transient shear stress in the rotational direction during OSP tests, suggesting that the shear rheology, and therefore, the structure of CB in the rotational direction is unaffected by the orthogonal oscillation.

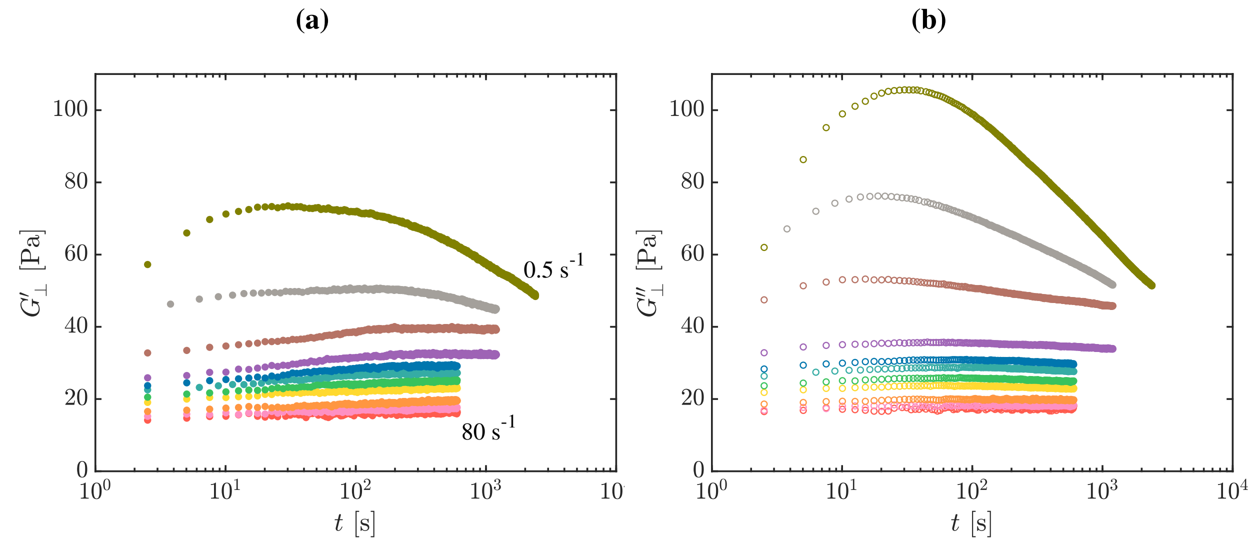


FIG. 8. The OSP results prove that the decay at long times comes from anti-thixotropy. The transient orthogonal (a) elastic and (b) viscous moduli of 4 wt% CB suspensions, measured by superposing an orthogonal oscillatory flow with 0.5% and 5 rad/s on the step-down shear rate flow in the rotational direction.

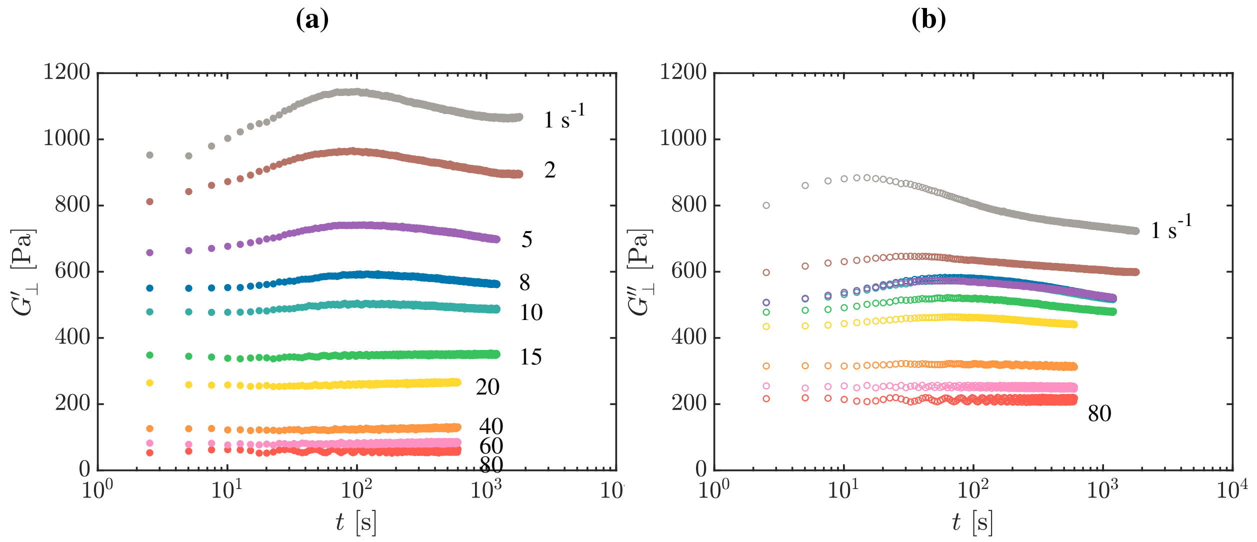


FIG. 9. The OSP results prove that the decay at long times comes from anti-thixotropy. The transient orthogonal (a) elastic and (b) viscous moduli of 8 wt% CB suspensions, measured by superposing an orthogonal oscillatory flow with 0.5% and 5 rad/s on the step-down shear rate flow in the rotational direction.

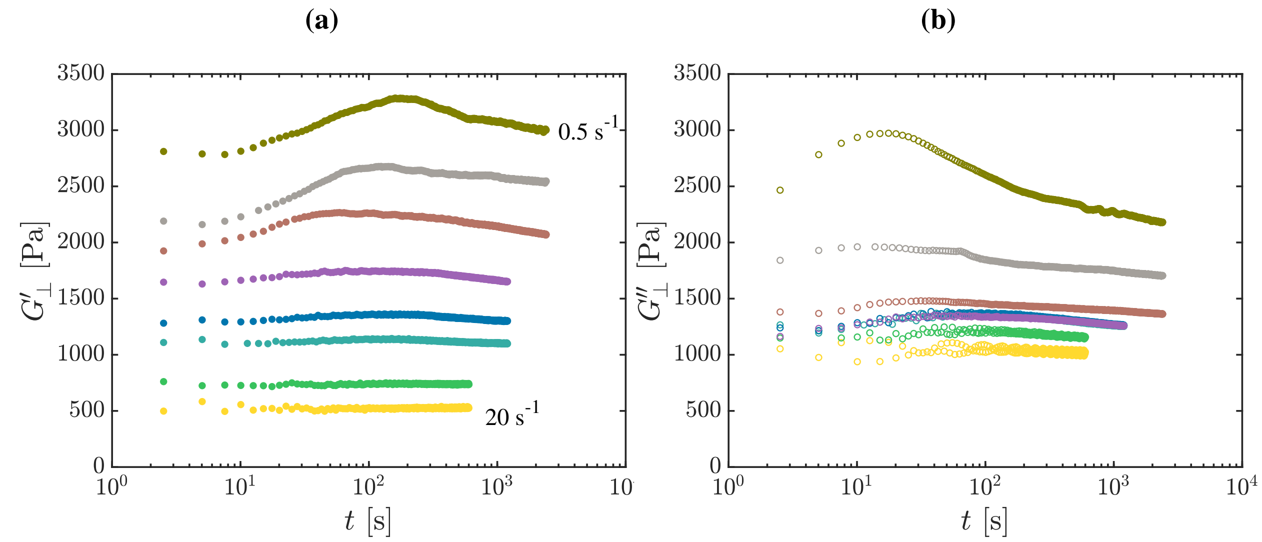


FIG. 10. The OSP results prove that the decay at long times comes from anti-thixotropy. The transient orthogonal (a) elastic and (b) viscous moduli of 10 wt% CB suspensions, measured by superposing an orthogonal oscillatory flow with 0.5% and 5 rad/s on the step-down shear rate flow in the rotational direction.

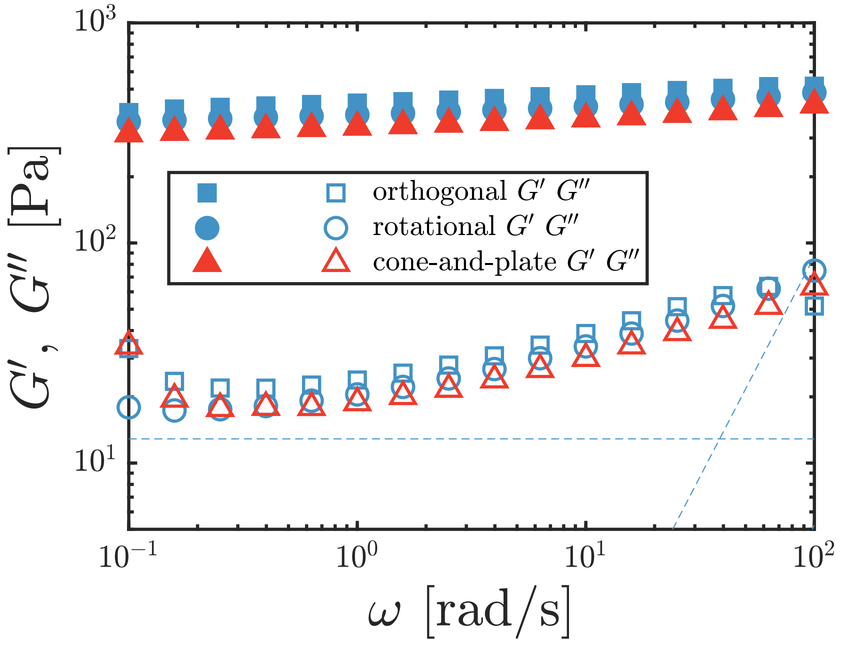


FIG. 11. A comparison of elastic and loss moduli of Carbopol measured by cone-and-plate, OSP geometry in rotational direction, and OSP in orthogonal direction.

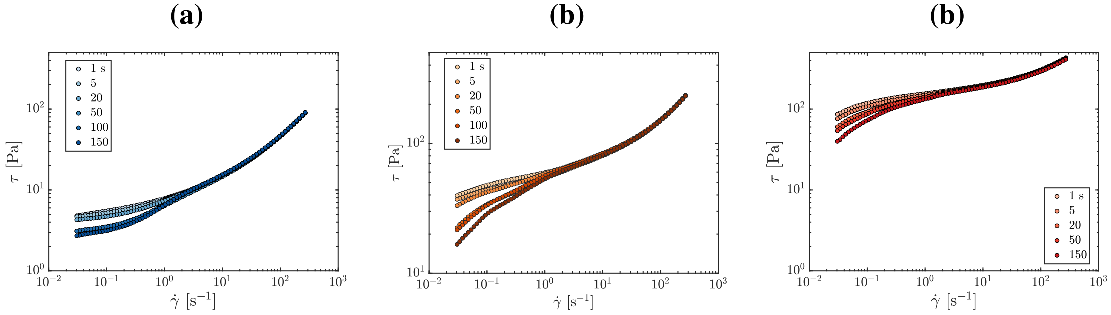


FIG. 12. The hysteresis loops measured with shear rate ramping down from 300 to 0.03 $s^{-1}$ was followed by an increasing ramp. Each ramp is performed in $n$ = 20 points per decade, and a different duration per point is used for each experiment.for CB suspensions of (a) 4 wt%; (b) 8 wt%; and (c) 10 wt%.
